# Supplementary material for: Generating Extended Resolution Proofs with a BDD-Based SAT Solver
Source: arXiv:2105.00885 source file (2023-03-27)
Supplement: Supplementary file 1 [file 06-appendix.tex]

\section{Measuring Program Performance}
\label{app:experimental-time}

\subsection{Reordered Parity Formulas}

\begin{figure}
\centering
\begin{tikzpicture}[scale = 1.0]
          \begin{axis}[mark options={scale=1},grid=both, grid style={black!10}, xmode=log, ymode=log, legend style={at={(0.95,0.40)}}, legend cell align={left},
                              x post scale=1.8, xlabel=$n$, xtick={4,16,64,256,1024,4096,16384}, xticklabels={$4$,$16$,$64$,$256$,$1024$,$4096$,$16384$},
                              xmin=4,xmax=16384,ymin=100,ymax=200000000, title={Parity Clauses}]
                              
\addplot[color=clearpurple, mark=square*, thick] coordinates { (4,415) (8,5252) (12,49935) (14,265404) (16,863979) (18,2051479) (19,7481486) (20,14899951) (21,27219246) (22,57601587)};
\addplot[only marks, color=midgreen, mark=x, thick] coordinates { (4,25) (4,25) (4,25) (4,25) (4,25) (8,110) (8,97) (8,242) (8,126) (8,118) (12,1478) (12,372) (12,363) (12,485) (12,778) (16,659) (16,1104) (16,3353) (16,1054) (16,3041) (20,11241) (20,12119) (20,90113) (20,7542) (20,9155) (24,11157) (24,8363) (24,8196) (24,10242) (24,14081) (28,39274) (28,10726371) (28,745715) (28,563725) (28,159690) (32,365070) (32,32821) (32,75527) (32,168719) (32,573882) (36,446329) (36,1151796) (36,8385340) (36,17798132) (36,20961911) (37,18703963) (37,8818834) (37,11103304) (37,3942440) (37,12918996) (38,16028053) (38,8369119) (38,16497620) (38,3396930) (38,4855311) (39,5681881) (39,29570325) (39,4835872) (39,6020027) (39,12354450) (40,4737359) (40,14070464) (40,5607629) (40,149370128) (41,1185420) (41,155012890) (41,16953784) (41,22921883) (42,5870786) (42,15652756) (42,32090940) (42,41334) (42,3719117) (43,48902092) (43,28033564) (43,51892217) (44,46250850) (44,67144407) (44,129182356) (44,39616354) (45,82131403) (45,29725948) (45,101414252) (45,122555435) (46,130391681) (47,21639233) (47,61770772) (47,166916134) (48,168600536) (48,181046037) (48,106156342) (49,101244119) (49,179297124) (50,162602527)};
\addplot[color=lightblue, mark=triangle, thick] coordinates { (4,461) (8,1681) (12,3522) (16,4991) (24,9141) (32,13735) (40,22945) (48,33806) (64,48501) (80,68082) (96,89019) (112,112314) (128,140992) (144,184099) (160,238021) (176,273015) (192,300894) (208,338954) (224,405755) (240,437765) (256,487404) (288,595214) (320,699579) (368,973759) (400,1167956) (432,1406691) (464,1600449) (496,1776241) (512,1878528) (576,2315844) (640,2858102) (704,3440772) (768,4110079) (832,4724980) (896,5689389) (960,6502192) (1024,7391283) (1100,8597975) (1200,10083918) (1300,11600733) (1400,13433626) (1500,15167593) (1600,17222932) (1700,19277215) (1800,21697340) (1900,24213888) (2000,26406004) (3000,61289257) (4000,106600023)};
\addplot[color=darkestblue, mark=pentagon*, thick] coordinates { (4,430) (8,2266) (12,4266) (16,6606) (24,10990) (32,20612) (40,24559) (48,34180) (64,51736) (80,57976) (96,94107) (112,133062) (128,132858) (144,176426) (160,227226) (176,248204) (192,251115) (208,279484) (224,317784) (240,465105) (256,410830) (288,559007) (320,503021) (368,787078) (400,862155) (432,1340399) (464,1324147) (496,1356069) (512,1486631) (576,1653477) (640,2446128) (704,2647618) (768,3112774) (832,3821618) (896,4011227) (960,4388784) (1000,4704381) (1024,4979097) (1100,6029403) (1200,7179716) (1300,7957617) (1400,9629902) (1500,10165254) (1600,12942687) (1700,13206323) (1800,14182703) (1900,17555815) (2000,18107956) (3000,40592272) (4000,67332210) (5000,109386150)};

            \legend{\scriptsize \textsf{Linear}, \scriptsize \textsf{\kissat{}}, \scriptsize \textsf{Bucket-Input}, \scriptsize \textsf{Bucket-Random}}
          \end{axis}
\end{tikzpicture}
\caption{Total number of clauses in proofs of reordered parity encodings with $n$ leaves (Subset of data from Figure~\protect{\ref{fig:data:parity}})}
\label{fig:data:parity-repeated}
\end{figure}

\begin{figure}
\centering
\begin{tikzpicture}[scale = 1.0]
          \begin{axis}[mark options={scale=1},grid=both, grid style={black!10}, xmode=log, ymode=log, legend style={at={(0.95,0.40)}}, legend cell align={left},
                              x post scale=1.8, xlabel=$n$, xtick={4,16,64,256,1024,4096,16384}, xticklabels={$4$,$16$,$64$,$256$,$1024$,$4096$,$16384$},
                              xmin=4,xmax=16384,ymin=1.0,ymax=10000, title={Seconds for Parity Proof Generation}]

\addplot[color=clearpurple, mark=square*, thick]  coordinates { (00004,2.9) (00008,4.48) (00012,6.24) (00014,12.32) (00016,36.62) (00018,56.38) (00019,288.63) (00020,596.6) (00021,1158.34) (00022,1708.9)};

\addplot[only marks, color=midgreen, mark=x, thick]  coordinates { (4,0.0) (4,0.0) (4,0.0) (4,0.0) (4,0.0) (8,0.0) (8,0.0) (8,0.0) (8,0.0) (8,0.0) (12,0.01) (12,0.0) (12,0.0) (12,0.0) (12,0.0) (16,0.0) (16,0.0) (16,0.01) (16,0.0) (16,0.01) (20,0.08) (20,0.08) (20,0.49) (20,0.03) (20,0.05) (24,0.07) (24,0.04) (24,0.04) (24,0.05) (24,0.09) (28,0.25) (28,102.85) (28,6.8) (28,4.16) (28,1.07) (32,2.85) (32,0.2) (32,0.49) (32,1.14) (32,4.26) (36,3.23) (36,10.31) (36,96.02) (36,189.09) (36,241.65) (37,269.12) (37,109.07) (37,146.02) (37,31.52) (37,145.4) (38,213.87) (38,95.37) (38,203.55) (38,36.47) (38,47.43) (39,62.73) (39,393.64) (39,38.38) (39,53.61) (39,134.83) (40,46.48) (40,3773.34) (40,213.2) (40,55.48) (40,2346.63) (41,12.08) (41,3083.07) (41,221.62) (41,3129.36) (41,299.91) (42,56.6) (42,208.8) (42,468.76) (42,0.27) (42,39.4) (43,3952.19) (43,914.65) (43,412.14) (43,767.73) (43,2837.08) (44,592.96) (44,4005.39) (44,1375.4) (44,1393.44) (44,540.8) (45,1301.5) (45,442.11) (45,1812.01) (45,2455.54) (45,2295.46) (46,2833.3) (46,4404.59) (46,4358.73) (46,2484.96) (46,2609.21) (47,266.15) (47,4535.68) (47,1016.66) (47,3221.11) (47,2721.71) (48,3939.42) (48,3486.31) (48,2124.17) (48,3574.72) (48,3832.71) (49,3844.36) (49,5718.18) (49,1721.66) (49,3182.71) (49,4070.54) (50,3794.6) (50,4455.01) (50,3202.73) (50,3051.07) (50,3517.4)};

\addplot[color=lightblue, mark=triangle, thick]  coordinates { (00004,3.76) (00008,3.54) (00012,3.81) (00016,4.06) (00024,4.14) (00032,4.03) (00040,3.99) (00048,4.41) (00064,4.69) (00080,5.02) (00096,5.5) (00112,5.92) (00128,6.46) (00144,7.47) (00160,8.56) (00176,9.38) (00192,9.85) (00208,10.84) (00224,11.97) (00240,12.67) (00256,13.79) (00288,16.06) (00320,18.46) (00368,24.54) (00400,28.54) (00432,36.79) (00464,41.09) (00496,45.22) (00512,47.58) (00576,58.41) (00640,73.61) (00704,87.03) (00768,107.03) (00832,123.04) (00896,149.35) (00960,172.65) (01024,198.81) (01100,232.4) (01200,277.28) (01300,326.49) (01400,383.29) (01500,443.12) (01600,515.42) (01700,583.24) (01800,658.54) (01900,750.52) (02000,837.54) (03000,2208.27) (04000,4456.42)};

\addplot[color=darkestblue, mark=pentagon*, thick]  coordinates { (00004,1.67) (00008,2.84) (00012,2.53) (00016,2.88) (00024,3.06) (00032,2.92) (00040,3.26) (00048,3.89) (00064,3.83) (00080,3.78) (00096,4.34) (00112,4.64) (00128,5.05) (00144,5.33) (00160,6.17) (00176,6.4) (00192,6.55) (00208,7.2) (00224,7.63) (00240,9.91) (00256,8.84) (00288,11.32) (00320,10.93) (00368,14.83) (00400,16.2) (00432,25.76) (00464,26.18) (00496,27.45) (00512,29.56) (00576,32.99) (00640,45.5) (00704,53.17) (00768,61.92) (00832,77.69) (00896,84.67) (00960,93.7) (01000,98.86) (01024,109.59) (01100,131.86) (01200,158.49) (01300,182.39) (01400,226.55) (01500,253.92) (01600,319.69) (01700,344.59) (01800,380.31) (01900,463.01) (02000,509.3) (02250,474.09) (02500,622.33) (02800,729.03) (03000,1394.72) (04000,2798.74) (05000,5298.05)};

            \legend{\scriptsize \textsf{Linear}, \scriptsize \textsf{\kissat{}}, \scriptsize \textsf{Bucket-Input}, \scriptsize \textsf{Bucket-Random}}
          \end{axis}
\end{tikzpicture}
\caption{Execution time (in seconds) when generating proofs of unsatisfiability}

\label{fig:data:parity-time}
\end{figure}  

\subsection{Mutilated Chessboard}

\begin{figure}
\centering
\begin{tikzpicture}[scale = 1.0]
          \begin{axis}[mark options={scale=1.0},grid=both, grid style={black!10}, xmode=log, ymode=log, legend style={at={(0.95,0.40)}}, legend cell align={left},
                              x post scale=1.8, xlabel=$n$, xtick={4,8,16,32,64,128}, xticklabels={$4$,$8$,$16$,$32$,$64$,$128$},xmin=4,xmax=160,ymin=1000,ymax=200000000, title={Mutilated Chessboard Proof Clauses}]
      
      \addplot[color=clearpurple, mark=pentagon*, thick] coordinates { (4, 1421) (8, 58569) (12, 2304439) (14, 13294319)};
      \addplot[color=bluegray, mark=triangle, thick] coordinates { (4, 1664) (8, 87341) (12, 1781947) (14, 7122851) (16, 27199819) (18, 100411697)};
      \addplot[color=clearorange, mark=x, thick] coordinates { (4, 1800) (8, 28574) (10, 88906) (12, 296082) (14, 1243646) (16, 5854281) (18, 22155680)};
      \addplot[color=midgreen, mark=o, very thick] coordinates { (4, 58) (6, 204) (8, 942) (10, 9180) (12, 48296) (14, 691551) (16, 4503635) (18, 17281161) (20, 65376268) (22, 136883320)};
      \addplot[color=redpurple, mark=diamond*, thick] coordinates { (4, 1493) (8, 12120) (12, 34830) (16, 72573) (20, 128268) (24, 204895) (28, 305414) (32, 432785) (36, 589968) (40, 779923) (44, 1005610) (48, 1269989) (52, 1576020) (56, 1926663) (60, 2324878) (64, 2773625) (68, 3275864) (72, 3834555) (76, 4452658) (80, 5133133) (84, 5878940) (88, 6693039) (92, 7578390) (96, 8537953) (100, 9574688) (104, 10691555) (108, 11891514) (112, 13177525) (116, 14552548) (120, 16019543) (124, 17581470) (128, 19241287) (140, 24837696) (150,30252390)};

            \legend{\scriptsize \textsf{No Quantification}, \scriptsize \textsf{Bucket}, \scriptsize \textsf{Linear}, \scriptsize \textsf{\textsc{kissat}}, \scriptsize \textsf{Column Scan}}
          \end{axis}
\end{tikzpicture}
\caption{Total number of clauses in proofs of $n \times n$ mutilated
  chess boards (Same data as Figure~\protect{\ref{fig:data:chess}})}

\label{fig:data:chess-repeated}
\end{figure}  

\begin{figure}
\centering
\begin{tikzpicture}[scale = 1.0]
          \begin{axis}[mark options={scale=1.0},grid=both, grid style={black!10}, xmode=log, ymode=log, legend style={at={(0.95,0.40)}}, legend cell align={left},
                              x post scale=1.8, xlabel=$n$, xtick={4,8,16,32,64,128}, xticklabels={$4$,$8$,$16$,$32$,$64$,$128$},xmin=4,xmax=160,ymin=1.0,ymax=50000, title={Seconds for Mutilated Chessboard Proof Generation}]

\addplot [color=clearpurple, mark=pentagon*, thick] coordinates { (4,0.05) (8,0.87) (12,42.37) (14,248.92)};
\addplot [color=bluegray, mark=triangle, thick] coordinates { (4,0.02) (8,1.26) (12,29.66) (14,130.21) (16,518.23) (18,2009.26)};
\addplot [color=clearorange, mark=x, thick] coordinates { (4,0.05) (8,0.45) (10,1.6) (12,6.31) (14,31.19) (16,160.34) (18,633.67)};
\addplot [color=midgreen, mark=o, very thick] coordinates { (8,0.01) (8,0.01) (10,0.11) (12,0.69) (14,13.81) (16,121.89) (18,780.77) (20,5240.84) (22,45343.1)};
\addplot [color=redpurple, mark=diamond*, thick] coordinates { (4,0.03) (8,0.25) (12,0.78) (16,1.76) (20,3.38) (24,6.03) (24,4.63) (28,10.13) (32,15.85) (36,24.53) (40,36.71) (44,53.88) (48,79.68) (52,109.7) (56,153.77) (60,213.23) (64,277.61) (68,381.77) (72,498.06) (76,657.53) (80,866.28) (84,1420.87) (88,1936.97) (92,3073.08) (96,4525.96) (100,1713.59) (104,2031.69) (108,2394.2) (112,2969.08) (116,3606.71) (120,4411.93) (124,5375.24) (128,6143.95) (140,10305.66) (150,16492.32)};

            \legend{\scriptsize \textsf{No Quantification}, \scriptsize \textsf{Bucket}, \scriptsize \textsf{Linear}, \scriptsize \textsf{\textsc{kissat}}, \scriptsize \textsf{Column Scan}}
          \end{axis}
\end{tikzpicture}
\caption{Execution time (in seconds) when generating proofs of unsatisfiability for mutilated chessboard.}

\label{fig:data:chess-time}
\end{figure}
